# Supplementary material for: Stochastic $k$-Center and $j$-Flat-Center Problems
Source: arXiv:1607.04989 source file (2016-09-10)
Supplement: Supplementary file 1 [file appendix.tex]

\section{Missing Details in Section~\ref{sec:coreset}}
\label{app:coreset}

\textbf{Lemma \ref{lm:totalsen}.}
Consider the weighted $j$-flat-median problem where $\calF$ is the set of all $j$-flats in $\R^d$. The total sensitivity of any weighted $n$-point set is $O(j^{1.5})$.

The proof of Lemma~\ref{lm:totalsen} is similar to that of Theorem 18 in~\cite{varadarajan2012sensitivity} except that we consider the weighted version. To prove Lemma~\ref{lm:totalsen}, we need the following lemma.

\begin{lemma}
\label{lm:planesen}
Consider the weighted $(d-1)$-flat-median problem where $\calF$ is the set of all hyperplanes in $\R^d$.  The total sensitivity of any weighted $n$-point set is $O(d^{1.5})$.
\end{lemma}

\begin{proof}
The proof is almost the same as Lemma 16 in~\cite{varadarajan2012sensitivity}. We first use a vector $u=[u_1,\ldots,u_{d+1}]^T$ in $\R^{d+1}$ to represent a hyperplane. Note that the hyperplane determined by $u$ is $F_u=\{x\in \R^d \mid \sum_{i\in [d]}u_i x_i+u_{d+1}=0\}$. Without loss of generality, we assume that $\sum_{i\in [d]}u_i^2=1$. It is not hard to see that for any point $s\in \R^d$, we have that $\dist(s,F_u)=|\sum_{i\in [d]}u_is_i+u_{d+1}|$.

Let $P=\{s_1,\ldots,s_n\}\subseteq \R^d$ be any set of $n$ weighted points with weight $w_i$. Let $\tilde{s_i}=[w_i s_i^T , w_i]$, which is different from the unweighted version. Let $M$ be the $n\times (d+1)$ matrix whose $i$th row is $\tilde{s_i}$. Note that $\dist(s_i,F_u)=|M_{i}u|$, where $M_i$ is the $i$th row of $M$. By Lemma 15 in~\cite{varadarajan2012sensitivity}, there is an $n\times (d+1)$ matrix $D$
\footnote{By Theorem 4 in~\cite{dasgupta2009sampling}, there is a linear time algorithm to compute the matrix $D$.}
which satisfies that: (1) $\sum_{i,j}|D_{ij}|\leq (d+1)^{1.5}$, (2) for all $u\in\R^{d+1}$ and any $i\in [n]$, we have $|M_i u|\leq \| D_i\|_1\|Mu\|_1$. Using this matrix $D$, we can see that the sensitivity of $s_i$ $\sigma_{P}(s_i)=\sup_{u}\frac{|M_iu|}{\|Mu\|}\leq \|D_i\|_1$. Thus, we can bound the total sensitivity
$$
\mathfrak{G}_{P}=\sum_{i\in [n]}\sigma_P(s_i)\leq \sum_{i\in [n]}\|D_i\|_1=\sum_{i,j}|D_{ij}|=(d+1)^{1.5},
$$
which finishes the proof.
\end{proof}

\begin{lemma}
\label{lm:dimreduction} Given an instance $P$ of a weighted $j$-flat-median problem in $\R^d$, let $F^*$ denote a shape that minimizes $\cost(P,F)$ over all $F\in \calF$. Let $s'$ denote $\proj(s,F^*)$ and let $P'$ denote $\proj(P,F^*)$.
\footnote{Here $\proj(s,F^*)$ is the projection of $s$ on $F^*$, and $\proj(P,F^*)$ denotes the multi-set $\{\proj(s,F^*)\|s\in P\}$.}
Assume that the distance function satisfies the relaxed triangle inequality: $\dist(s,t)\leq \alpha(\dist(s,r)+\dist(r,t))$ for any $s,t,r\in \R^d$ for some constant $\alpha\geq 1$. Then
\begin{enumerate}
\item The following inequality holds: $\mathfrak{G}_P\leq 2\alpha^2\mathfrak{G}_{P'}+\alpha$.
\item If $\cost(P,F^*)=0$, then $\sigma_P(s)=\sigma_{P'}(s')$ for each $s\in P$. If $\cost(P,F^*)>0$, then $\sigma_P(s)\leq \alpha\frac{\cost(s,s')}{\cost(P,F^*)}+2\alpha^2\sigma_{P'}(s')$.
\end{enumerate}
\end{lemma}

Note that Lemma~\ref{lm:dimreduction} is almost the same as Theorem 7 in~\cite{varadarajan2012sensitivity} except that we consider the weighted version. The main difference is that we replace function $\dist(\cdot,\cdot)$ by $\cost(\cdot,\cdot)$ in the weighted version, which does not affect the correctness of the lemma. In fact, the Euclidean distance function $\dist()$ satisfies the triangle inequality. So we can set $\alpha=1$ in Lemma~\ref{lm:dimreduction}.

Now we are ready to prove Lemma~\ref{lm:totalsen}.

\begin{proofoflm}{\ref{lm:totalsen}}
By Lemma~\ref{lm:dimreduction}, we project the instance $\calP$ to the optimal $j$-flat $F^*$. Note that the projected point set $\calP'$ is contained in a $j$-flat. Furthermore, each shape is a $j$-flat. So we reduce the weighted $j$-flat-median problem to an $O(j)$-dimensional subspace. By Corollary 17 in~\cite{varadarajan2012sensitivity}, we know that the sensitivity of each weighted point for $j$-flats is no more than that for hyperplanes. So does the total sensitivity. Thus, we can bound $\mathfrak{G}_P$ for any weighted instance $P$ by $O(j^{1.5})$ using Lemma~\ref{lm:planesen}.
\end{proofoflm}
